# Supplementary material for: Jamming-controlled stochasticity in metal-insulator switching
Source: arXiv:2602.11302 ancillary file (2026-02-11)
Supplement: Supplementary file 1 [file supplement.pdf]

# Supplemental Information: Jamming-controlled stochasticity in metal-insulator switching

Nicolò D'Anna,<sup>1,\*</sup> Nareg Ghazikhanian,<sup>1</sup> Katherine Matthews,<sup>1</sup> Daseul Ham,<sup>2</sup> Su Yong Lee,<sup>2</sup> Alex Frano,<sup>1</sup> Ivan K. Schuller,<sup>1</sup> and Oleg Shpyrko<sup>1</sup>

<sup>1</sup>*University of California San Diego, La Jolla, CA 92093, USA*

<sup>2</sup>*Pohang Light Source-II (PLS-II) Beamline Department,  
Pohang Accelerator Laboratory, POSTECH, Pohang 37673, Republic of Korea*

---

\* ndanna@ucsd.edu

### Results from the pristine device at 60 °C

*Domain dynamics in response to electric fields:* Correlation decay of sub-threshold (0.24 mA) electrical switching of the pristine device is shown in Fig. 1a and ???. It is marked by a slow erasure of the initial nano-domain distribution on timescales  $\approx 1000$  s, analogous the to the device discussed in the main article.

Repetitive above-threshold (1 mA) electrical switching with a period of 3 s is shown in Fig. ?? and 1d. The same plastic learning behavior is observed as with the device discussed in the main article. The initial 400 switching events are more stochastic, then the switching gradually becomes more deterministic until it reaches a maximum at  $\sim 1000$  cycles.

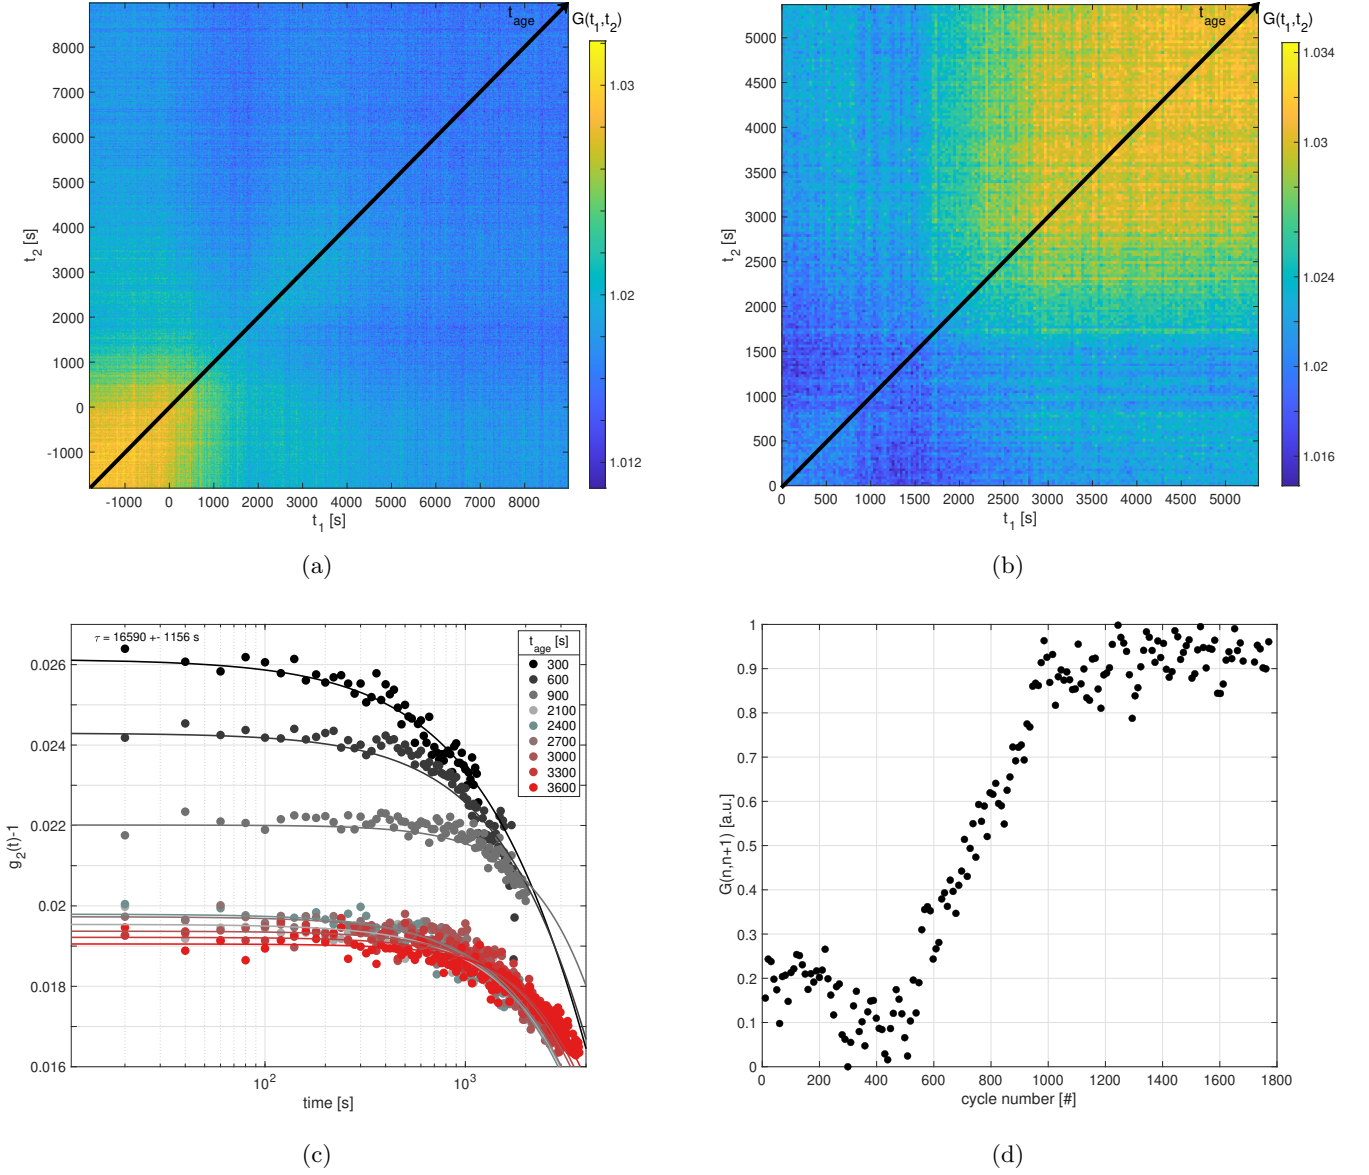

FIG. 1: **Electrical switching of a pristine device at 60 °C.** (a) Two-times correlation while a 0.24 mA sub-threshold current is turned on ( $t = 0$  s). (b) Two-times correlation while repetitively forming the percolating filament with an above-threshold current of 1 mA. (c)  $t_{age}$  dependent one time correlation  $g_2(t)$  obtained from (a). (d) Correlation  $G(n, n+1)$  between cycle  $n$  and  $n+1$ , obtained from the data in (b).

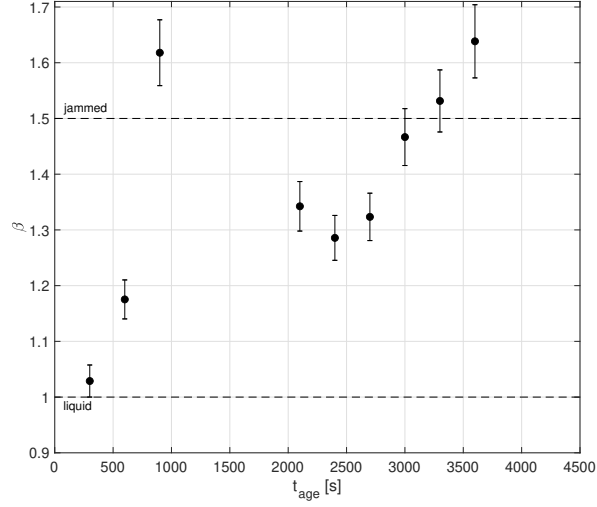

FIG. 2: **Jamming transition.** Stretching exponent as a function of  $t_{\text{age}}$ , obtained from fitting the data in Fig. 1c.

*Electrically driven jamming transition:* The correlation decay data from Fig. 1a are fitted with the exponential decay  $|F_{t_{\text{age}}}(t)| = \exp(-(t/\tau)^\beta)$ . The data for  $t_{\text{age}} > 4000$  s is not fitted, because the decay was too small to obtain good fits. The stretching exponent  $\beta$  is shown as a function of  $t_{\text{age}}$  in Fig. 2. The jamming transition from  $\beta = 1$  to  $\beta = 1.5$  is observed in the pristine  $V=2$  device.

*Electrical Measurements:* Electrical transport measurements were performed in the four-probe station during the XPCS beamtime. Temperature dependence of the pristine device resistance is shown in Fig. 3a. Electrical switching at 60 °C is shown in Fig. 3b, with  $I_1$  indicating the switching threshold current. The sub-threshold and above-threshold currents used for Fig. 1 were 0.24 mA and 1 mA, respectively.

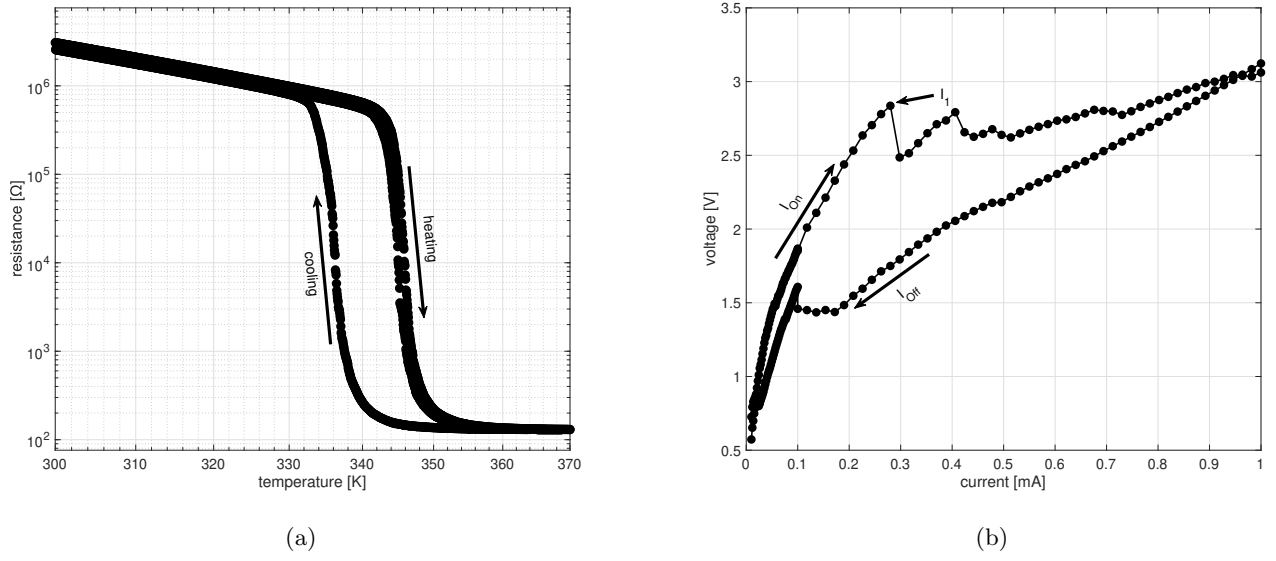

FIG. 3: **Resistance measurements of a pristine device.** (a) Resistance versus temperature. (b) Voltage versus current.
